# Supplementary material for: The Category Theoretic Solution of Recursive Program Schemes
Source: arXiv:0904.2385 ancillary file (2009-04-15)
Supplement: Supplementary file 1 [file slides.pdf]

# Coalgebras, Monads and Semantics

Stefan Milius

`milius@iti.cs.tu-bs.de`

Institut für Theoretische Informatik  
Technische Universität Carolo-Wilhelmina  
zu Braunschweig

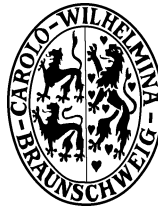

# Outline

1. Coalgebras as models of systems
2. Monads of final coalgebras
3. Coalgebraic semantics of recursive function definitions
4. Applications

# 1. (Co)algebras for a functor

**Definition.** Consider an endofunctor  $H : \text{Set} \longrightarrow \text{Set}$ .

$H$ -algebra

$$HA \xrightarrow{\alpha} A$$

$A$  – “data”  
 $\alpha$  – “operations”

$H$ -coalgebra

$$A \xrightarrow{\alpha} HA$$

$A$  – “states”  
 $\alpha$  – “reactions”

# 1. (Co)algebras for a functor

**Definition.** Consider an endofunctor  $H : \text{Set} \longrightarrow \text{Set}$ .

$H$ -algebra homomorphism

$$\begin{array}{ccc} HA & \xrightarrow{\alpha} & A \\ Hf \downarrow & & \downarrow f \\ HB & \xrightarrow{\beta} & B \end{array} \quad \begin{array}{l} A - \text{“data”} \\ \alpha - \text{“operations”} \end{array}$$

$H$ -coalgebra homomorphism

$$\begin{array}{ccc} A & \xrightarrow{\alpha} & HA \\ f \downarrow & & \downarrow Hf \\ B & \xrightarrow{\beta} & HB \end{array} \quad \begin{array}{l} A - \text{“states”} \\ \alpha - \text{“reactions”} \end{array}$$

# 1. (Co)algebras for a functor

**Definition.** Consider an endofunctor  $H : \text{Set} \longrightarrow \text{Set}$ .

$H$ -algebra homomorphism

$$\begin{array}{ccc} HA & \xrightarrow{\alpha} & A \\ Hf \downarrow & & \downarrow f \\ HB & \xrightarrow{\beta} & B \end{array} \quad \begin{array}{l} A - \text{“data”} \\ \alpha - \text{“operations”} \end{array}$$

$H$ -coalgebra homomorphism

$$\begin{array}{ccc} A & \xrightarrow{\alpha} & HA \\ f \downarrow & & \downarrow Hf \\ B & \xrightarrow{\beta} & HB \end{array} \quad \begin{array}{l} A - \text{“states”} \\ \alpha - \text{“reactions”} \end{array}$$

## Examples of Algebras

| Functor                                                                                                                                            | Algebras                                                                                           |
|----------------------------------------------------------------------------------------------------------------------------------------------------|----------------------------------------------------------------------------------------------------|
| $HX = 1 + X \times X$                                                                                                                              | $1 \longrightarrow A \longleftarrow A \times A$<br>algebras with a binary operation and a constant |
| $\Sigma = (\Sigma_n)_{n \in \mathbb{N}}$ signature $\rightsquigarrow$<br>$H_\Sigma X = \Sigma_0 + \Sigma_1 \times X + \Sigma_2 \times X^2 + \dots$ | algebras for the signature $\Sigma$                                                                |

J. Adámek and V. Trnkova, *Automata and Algebras in Categories*, Kluwer 1990.

# Systems, systems, systems, ...

Jan Rutten, Universal Coalgebra: a theory of systems, TCS 249 (2000).

| Functor                    | Coalgebra                               | Description                                        |
|----------------------------|-----------------------------------------|----------------------------------------------------|
| $HX = \mathbb{R} \times X$ | $A \longrightarrow \mathbb{R} \times A$ | deterministic automata with output in $\mathbb{R}$ |

# Systems, systems, systems, ...

Jan Rutten, Universal Coalgebra: a theory of systems, TCS 249 (2000).

| Functor                         | Coalgebra                                    | Description                                          |
|---------------------------------|----------------------------------------------|------------------------------------------------------|
| $HX = \mathbb{R} \times X$      | $A \longrightarrow \mathbb{R} \times A$      | deterministic automata with output in $\mathbb{R}$   |
| $HX = \{0, 1\} \times X^\Sigma$ | $A \longrightarrow \{0, 1\} \times A^\Sigma$ | deterministic acceptors with input alphabet $\Sigma$ |

Jan Rutten, Automata and coinduction (an exercise in coalgebra), LNCS 1466, 1998.

# Systems, systems, systems, ...

Jan Rutten, Universal Coalgebra: a theory of systems, TCS 249 (2000).

| Functor                         | Coalgebra                                    | Description                                          |
|---------------------------------|----------------------------------------------|------------------------------------------------------|
| $HX = \mathbb{R} \times X$      | $A \longrightarrow \mathbb{R} \times A$      | deterministic automata with output in $\mathbb{R}$   |
| $HX = \{0, 1\} \times X^\Sigma$ | $A \longrightarrow \{0, 1\} \times A^\Sigma$ | deterministic acceptors with input alphabet $\Sigma$ |
| $HX = \mathcal{P}(X)$           | $A \longrightarrow \mathcal{P}(A)$           | graphs (+ edge reflecting homomorphisms)             |



# Systems, systems, systems, ...

Jan Rutten, Universal Coalgebra: a theory of systems, TCS 249 (2000).

| Functor                                 | Coalgebra                                            | Description                                          |
|-----------------------------------------|------------------------------------------------------|------------------------------------------------------|
| $HX = \mathbb{R} \times X$              | $A \longrightarrow \mathbb{R} \times A$              | deterministic automata with output in $\mathbb{R}$   |
| $HX = \{0, 1\} \times X^\Sigma$         | $A \longrightarrow \{0, 1\} \times A^\Sigma$         | deterministic acceptors with input alphabet $\Sigma$ |
| $HX = \mathcal{P}(X)$                   | $A \longrightarrow \mathcal{P}(A)$                   | graphs (+ edge reflection homomorphisms)             |
| $HX = \mathcal{P}(\text{Act} \times X)$ | $A \longrightarrow \mathcal{P}(\text{Act} \times A)$ | labelled transition systems                          |

# Systems, systems, systems, ...

Jan Rutten, Universal Coalgebra: a theory of systems, TCS 249 (2000).

| Functor                                 | Coalgebra                                            | Description                                                   |
|-----------------------------------------|------------------------------------------------------|---------------------------------------------------------------|
| $HX = \mathbb{R} \times X$              | $A \longrightarrow \mathbb{R} \times A$              | deterministic automata with output in $\mathbb{R}$            |
| $HX = \{0, 1\} \times X^\Sigma$         | $A \longrightarrow \{0, 1\} \times A^\Sigma$         | deterministic acceptors with input alphabet $\Sigma$          |
| $HX = \mathcal{P}(X)$                   | $A \longrightarrow \mathcal{P}(A)$                   | graphs (+ edge reflection homomorphisms)                      |
| $HX = \mathcal{P}(\text{Act} \times X)$ | $A \longrightarrow \mathcal{P}(\text{Act} \times A)$ | labelled transition systems                                   |
| $H_\Sigma X = 1 + X \times X$           | $A \longrightarrow 1 + A \times A$                   | automata with binary input and halting states                 |
| $HX = H_\Sigma X$                       | $A \longrightarrow H_\Sigma A$                       | automata with output in $\Sigma$ and input according to arity |

# Systems, systems, systems, ...

Jan Rutten, Universal Coalgebra: a theory of systems, TCS 249 (2000).

| Functor                                 | Coalgebra                                            | Description                                                   |
|-----------------------------------------|------------------------------------------------------|---------------------------------------------------------------|
| $HX = \mathbb{R} \times X$              | $A \longrightarrow \mathbb{R} \times A$              | deterministic automata with output in $\mathbb{R}$            |
| $HX = \{0, 1\} \times X^\Sigma$         | $A \longrightarrow \{0, 1\} \times A^\Sigma$         | deterministic acceptors with input alphabet $\Sigma$          |
| $HX = \mathcal{P}(X)$                   | $A \longrightarrow \mathcal{P}(A)$                   | graphs (+ edge reflection homomorphisms)                      |
| $HX = \mathcal{P}(\text{Act} \times X)$ | $A \longrightarrow \mathcal{P}(\text{Act} \times A)$ | labelled transition systems                                   |
| $H_\Sigma X = 1 + X \times X$           | $A \longrightarrow 1 + A \times A$                   | automata with binary input and halting states                 |
| $HX = H_\Sigma X$                       | $A \longrightarrow H_\Sigma A$                       | automata with output in $\Sigma$ and input according to arity |

**Other examples:** Kripke models  
Probabilistic transition systems  
etc.

# Final Coalgebras

**Definition.** final  $H$ -coalgebra

$$T \xrightarrow[t]{} HT$$

# Final Coalgebras

**Definition.** final  $H$ -coalgebra

$$\begin{array}{ccc} A & \xrightarrow[\alpha]{\forall} & HA \\ \exists! f \downarrow \text{dotted} & & \downarrow Hf \\ T & \xrightarrow{t} & HT \end{array}$$

# Final Coalgebras

**Definition.** final  $H$ -coalgebra

$$\begin{array}{ccc} A & \xrightarrow[\alpha]{\forall} & HA \\ \downarrow \exists! f & & \downarrow Hf \\ T & \xrightarrow{t} & HT \end{array}$$

- **Lambek's Lemma.**  $t : T \longrightarrow HT$  is an isomorphism.
- final coalgebras exist for a large class of endofunctors  
(e. g. all accessible endofunctors of Set)  
P. Aczel and N. Mendler (1989); M. Barr (1993); J. Worrell (2005);  
J. Adámek, J. Velebil, SM (2004).
- generic notion of **bisimulation**
- $T =$  all behaviours of systems of type  $H$  modulo largest bisimulation.

# Final Coalgebras – Examples

| Functor                                                          | Final Coalgebra                                                                                                                     |
|------------------------------------------------------------------|-------------------------------------------------------------------------------------------------------------------------------------|
| $HX = \mathbb{R} \times X$                                       | streams of real numbers: $\mathbb{R}^\omega \xrightarrow{\langle \text{hd}, \text{tl} \rangle} \mathbb{R} \times \mathbb{R}^\omega$ |
| $HX = \{0, 1\} \times X^\Sigma$                                  | $\mathcal{P}(\Sigma^*) = \text{formal languages over } \Sigma$                                                                      |
| $HX = \mathcal{P}(X)$<br>$HX = \mathcal{P}(\text{Act} \times X)$ | does not exist – but one can work in classes                                                                                        |
| $H_\Sigma X = 1 + X \times X$                                    | finite and infinite binary trees<br><br>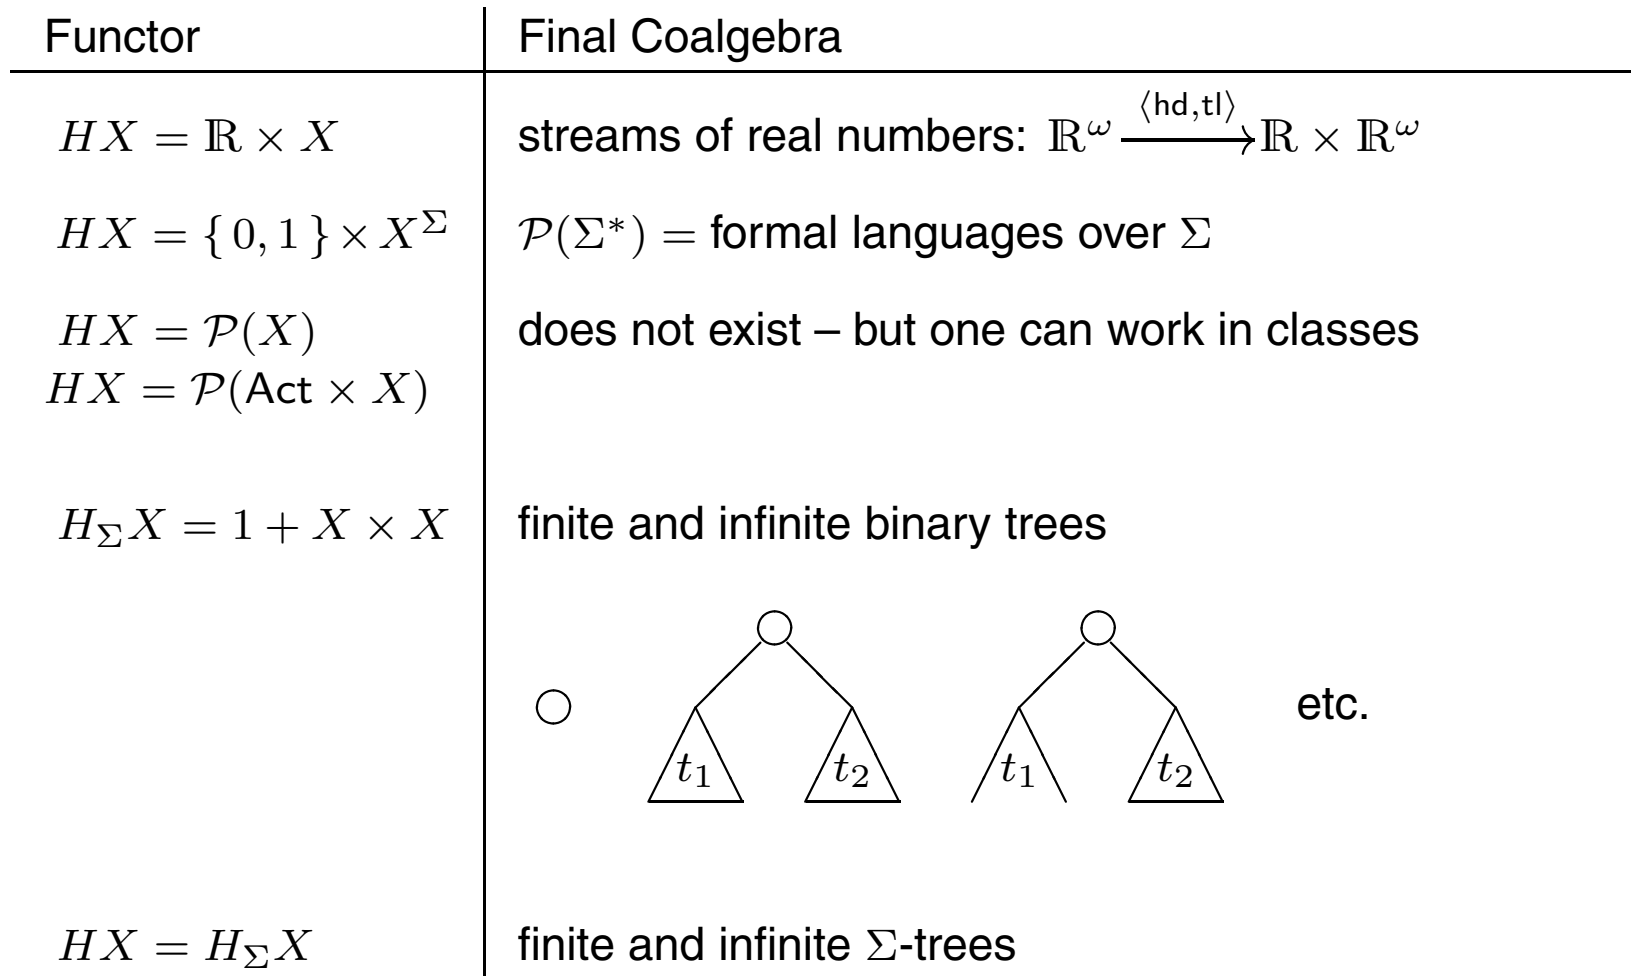         |
| $HX = H_\Sigma X$                                                | finite and infinite $\Sigma$ -trees                                                                                                 |

# Some Topics in Coalgebra

- Logic and Coalgebra: modal logics as specification languages for coalgebras:  
L. Moss, Coalgebraic Modal Logic, Ann. Pure Appl. Logic, 1999;  
A. Baltag, C. Cirstea, A. Kurz, D. Pattinson . . .



# Some Topics in Coalgebra

- Logic and Coalgebra: modal logics as specification languages for coalgebras:  
L. Moss, Coalgebraic Modal Logic, Ann. Pure Appl. Logic, 1999;  
A. Baltag, C. Cirstea, A. Kurz, D. Pattinson . . .
- Mathematical foundations of operational semantics:  
D. Turi, G. Plotkin, J. Rutten, M. Lenisa, H. Watanabe, J. Power, F. Bartels, . . .

# Some Topics in Coalgebra

- Logic and Coalgebra: modal logics as specification languages for coalgebras:  
L. Moss, Coalgebraic Modal Logic, Ann. Pure Appl. Logic, 1999;  
A. Baltag, C. Cirstea, A. Kurz, D. Pattinson . . .
- Mathematical foundations of operational semantics:  
D. Turi, G. Plotkin, J. Rutten, M. Lenisa, H. Watanabe, J. Power, F. Bartels, . . .
- Semantics of Recursion  
L. Moss, Parametric Corecursion, TCS 260 (2001)  
N. Ghani, C. Lüth, F. De Marchi; T. Uustalu; J. Adámek, J. Velebil and SM

# Some Topics in Coalgebra

- Logic and Coalgebra: modal logics as specification languages for coalgebras:  
L. Moss, Coalgebraic Modal Logic, Ann. Pure Appl. Logic, 1999;  
A. Baltag, C. Cirstea, A. Kurz, D. Pattinson . . .
- Mathematical foundations of operational semantics:  
D. Turi, G. Plotkin, J. Rutten, M. Lenisa, H. Watanabe, J. Power, F. Bartels, . . .
- Semantics of Recursion  
L. Moss, Parametric Corecursion, TCS 260 (2001)  
N. Ghani, C. Lüth, F. De Marchi; T. Uustalu; J. Adámek, J. Velebil and SM
- Applications  
J. Rutten: stream calculus  
B. Jacobs et al.: semantics of object oriented programming languages  
Coalgebraic specification languages + tool support (e. g. CoCASL by T. Mossakowski,  
L. Schröder et al.)

etc.

## 2. Monads of Final Coalgebras

**Classical Result** of Calvin Elgot et al. (1978)

Infinite trees over a signature  $\Sigma$  form the free completely iterative theory on  $\Sigma$ .

## 2. Monads of Final Coalgebras

**Classical Result** of Calvin Elgot et al. (1978)

Infinite trees over a signature  $\Sigma$  form the free completely iterative theory on  $\Sigma$ .

|                                                     |                    |                                                                             |
|-----------------------------------------------------|--------------------|-----------------------------------------------------------------------------|
| signatures $\Sigma = (\Sigma_n)_{n \in \mathbb{N}}$ | $\rightsquigarrow$ | polynomial endofunctors $H_\Sigma : \text{Set} \longrightarrow \text{Set};$ |
| (in)finite trees $T_\Sigma X$                       | $\rightsquigarrow$ | final coalgebra for $H_\Sigma(-) + X$                                       |

### Assumptions.

- (i)  $\mathcal{A}$  category with  $+$  (and with monomorphic injections)
- (ii) we use endofunctors  $H : \mathcal{A} \longrightarrow \mathcal{A}$  with **enough final coalgebras**:

$$\forall X \quad \exists \quad TX \xrightarrow{\alpha_X} HTX + X \quad \text{final coalgebra for } H(-) + X$$

# Substitution

## Notation.

$T \xrightarrow{\alpha} HT + Id$   
is an isomorphism

$\Rightarrow$

$$\left. \begin{array}{l} \eta: Id \longrightarrow T \\ \tau: HT \longrightarrow T \end{array} \right\} \text{coproduct injections}$$

# Substitution

## Notation.

$$\begin{array}{l}
 T \xrightarrow{\alpha} HT + Id \\
 \text{is an isomorphism}
 \end{array}
 \implies
 \left. \begin{array}{l}
 \eta: Id \longrightarrow T \\
 \tau: HT \longrightarrow T
 \end{array} \right\} \text{coproduct injections}$$

**Proposition.**  $\forall s : X \longrightarrow TY \quad \exists! \hat{s} : TX \longrightarrow TY$  such that

$$\begin{array}{ccccc}
 X & \xrightarrow{\eta_X} & TX & \xleftarrow{\tau_X} & HTX \\
 & \searrow s & \downarrow \hat{s} & & \downarrow H\hat{s} \\
 & & TY & \xleftarrow{\tau_Y} & HTY
 \end{array}$$

# Substitution

## Notation.

$$\left. \begin{array}{l} T \xrightarrow{\alpha} HT + Id \\ \text{is an isomorphism} \end{array} \right\} \Rightarrow \left. \begin{array}{l} \eta: Id \longrightarrow T \\ \tau: HT \longrightarrow T \end{array} \right\} \text{coproduct injections}$$

**Proposition.**  $\forall s : X \longrightarrow TY \quad \exists! \hat{s} : TX \longrightarrow TY$  such that

$$\begin{array}{ccccc} X & \xrightarrow{\eta_X} & TX & \xleftarrow{\tau_X} & HTX \\ & \searrow s & \downarrow \hat{s} & & \downarrow H\hat{s} \\ & & TY & \xleftarrow{\tau_Y} & HTY \end{array}$$

**Theorem.** (Aczel, Adamek, Velebil, SM)

- (i)  $T$  is the object assignment of a monad;
- (ii) this monad is the **free** completely iterative monad on  $H$ .

Freeness  $\rightsquigarrow$  abstract version of *second-order* substitution  
(= substitution of trees for operation symbols)



# 3. Semantics of Recursive Function Definitions

$$\varphi(x) \approx F(x, \varphi(Gx))$$

$F, G$     **givens** from a signature  $\Sigma$   
 $\varphi$     from a signature  $\Phi$

# 3. Semantics of Recursive Function Definitions

$$\varphi(x) \approx F(x, \varphi(Gx))$$

$F, G$     **givens** from a signature  $\Sigma$   
 $\varphi$     from a signature  $\Phi$

## Uninterpreted Semantics

$$\varphi^\dagger(x) =$$

```
graph TD; F1[F] --- x[x]; F1 --- F2[F]; F2 --- Gx[Gx]; F2 --- F3[F]; F3 --- GGx[GGx]; F3 -.- dots[...];
```

# 3. Semantics of Recursive Function Definitions

$$\varphi(x) \approx F(x, \varphi(Gx))$$

$$\Sigma\text{-algebra } A: \quad A \times A \xrightarrow{F_A} A$$

$F, G$     **givens** from a signature  $\Sigma$     **and**  
 $\varphi$     from a signature  $\Phi$

$$A \xrightarrow{G_A} A$$

## Uninterpreted Semantics

$$\varphi^\dagger(x) =$$

```

    F
   / \
  x   F
     / \
    Gx  F
       / \
      GGx ...
    
```

# 3. Semantics of Recursive Function Definitions

$$\varphi(x) \approx F(x, \varphi(Gx))$$

$$\Sigma\text{-algebra } A: \quad A \times A \xrightarrow{F_A} A$$

$F, G$  **givens** from a signature  $\Sigma$  **and**  
 $\varphi$  from a signature  $\Phi$

$$A \xrightarrow{G_A} A$$

## Uninterpreted Semantics

$$\varphi^\dagger(x) =$$

## Interpreted Semantics

a unary Operation  $\varphi_A : A \longrightarrow A$  with

$$\varphi_A(a) = F_A(a, \varphi_A(G_A(a)))$$

I. Guessarian, *Algebraic Semantics*, Springer 1981.

# Problems

- What is a recursive program scheme?
- What is a *solution* of a recursive program scheme?
- What algebras are suitable for interpreted semantics?
- How to find (un)interpreted solutions?

# Recursive Program Schemes Categorically

## Classically:

$\Sigma$       signature of given functions;       $\Phi$       signature of recursively defined functions  
system of formal equations

$$f(x_1, \dots, x_n) \approx t^f(x_1, \dots, x_n), \quad f \in \Phi_n, \quad n \in \mathbb{N}.$$

$\uparrow$   
terms/trees over  $\Sigma + \Phi$

# Recursive Program Schemes Categorically

## Classically:

$\Sigma$  signature of given functions;       $\Phi$  signature of recursively defined functions  
system of formal equations

$$f(x_1, \dots, x_n) \approx t^f(x_1, \dots, x_n), \quad f \in \Phi_n, \quad n \in \mathbb{N}.$$

$\uparrow$   
terms/trees over  $\Sigma + \Phi$

**Categorically:** signatures **are** functors:       $\Sigma, \Phi : \mathbb{N} \longrightarrow \text{Set}$        $\mathbb{N}$  discrete category

formal equations **are** natural transformations:

$$\Phi_n \longrightarrow T_{\Sigma + \Phi} \{ 0, \dots, n - 1 \} \quad \forall n$$

# Recursive Program Schemes Categorically

## Classically:

$\Sigma$  signature of given functions;  $\Phi$  signature of recursively defined functions  
system of formal equations

$$f(x_1, \dots, x_n) \approx t^f(x_1, \dots, x_n), \quad f \in \Phi_n, \quad n \in \mathbb{N}.$$

$\uparrow$   
 terms/trees over  $\Sigma + \Phi$

## Categorically: signatures **are** functors:

$\Sigma, \Phi : \mathbb{N} \longrightarrow \text{Set}$   $\mathbb{N}$  discrete category

formal equations **are** natural transformations:

|                      |                   |                                               |
|----------------------|-------------------|-----------------------------------------------|
| $\Phi_n$             | $\longrightarrow$ | $T_{\Sigma+\Phi} \{0, \dots, n-1\} \forall n$ |
| $\Phi$               | $\longrightarrow$ | $T_{\Sigma+\Phi} \cdot J$                     |
| $\text{Lan}_J(\Phi)$ | $\longrightarrow$ | $T_{\Sigma+\Phi}$                             |
| $H_\Phi$             | $\longrightarrow$ | $T^{H_\Sigma+H_\Phi}$                         |

$$J : \mathbb{N} \longrightarrow \text{Set}, \quad n \longmapsto \{0, \dots, n-1\}$$

$$\text{Lan}_J(-) \dashv (-) \cdot J$$

$$\text{Notation: } H \rightsquigarrow T^H, \quad K \rightsquigarrow T^K \text{ etc.}$$



# Recursive Program Schemes Categorically

## Classically:

$\Sigma$  signature of given functions;       $\Phi$  signature of recursively defined functions  
system of formal equations

$$f(x_1, \dots, x_n) \approx \underset{\substack{\uparrow \\ \text{terms/trees over } \Sigma + \Phi}}{t^f(x_1, \dots, x_n)}, \quad f \in \Phi_n, \quad n \in \mathbb{N}.$$

## Categorically: signatures **are** functors:

$\Sigma, \Phi : \mathbb{N} \longrightarrow \text{Set}$        $\mathbb{N}$  discrete category

formal equations **are** natural transformations:

|                      |                   |                                               |
|----------------------|-------------------|-----------------------------------------------|
| $\Phi_n$             | $\longrightarrow$ | $T_{\Sigma+\Phi} \{0, \dots, n-1\} \forall n$ |
| $\Phi$               | $\longrightarrow$ | $T_{\Sigma+\Phi} \cdot J$                     |
| $\text{Lan}_J(\Phi)$ | $\longrightarrow$ | $T_{\Sigma+\Phi}$                             |
| $H_\Phi$             | $\longrightarrow$ | $T^{H\Sigma+H\Phi}$                           |

$$J : \mathbb{N} \longrightarrow \text{Set}, \quad n \longmapsto \{0, \dots, n-1\}$$

$$\text{Lan}_J(-) \dashv (-) \cdot J$$

$$\text{Notation: } H \rightsquigarrow T^H, \quad K \rightsquigarrow T^K \text{ etc.}$$

**Definition.** A recursive program scheme (**RPS**) is a natural transformation

$$V \longrightarrow T^{H+V}$$

$$H : \mathcal{A} \longrightarrow \mathcal{A} \quad \text{“givens”}$$

$$V : \mathcal{A} \longrightarrow \mathcal{A} \quad \text{“variables”}$$

# Uninterpreted RPS Solutions

**Definition.** A solution of an RPS  $e : V \longrightarrow T^{H+V}$  is a natural transformation

$$e^\dagger : V \longrightarrow T^H \quad \text{Note: } \frac{H_\Phi \longrightarrow T^{H\Sigma}}{\Phi_n \longrightarrow T_\Sigma\{0, \dots, n-1\} \forall n}$$

such that “ $e^\dagger$  is a fixed-point w. r. t. second-order substitution.”

# Uninterpreted RPS Solutions

**Definition.** A solution of an RPS  $e : V \longrightarrow T^{H+V}$  is a natural transformation

$$e^\dagger : V \longrightarrow T^H \quad \text{Note: } \frac{H_\Phi \longrightarrow T^{H\Sigma}}{\Phi_n \longrightarrow T_\Sigma\{0, \dots, n-1\} \forall n}$$

such that “ $e^\dagger$  is a fixed-point w. r. t. second-order substitution.”

**Theorem.** Every *guarded* RPS has a unique solution.

**Guardedness.**  $\varphi(x) \approx \varphi(x)$  has no unique solution

“each right-hand side starts with a given operation”  
can be easily expressed categorically

# Example: Classical Uninterpreted Semantics

**RPS**

$$f(n) \approx \text{ifzero}(n, \text{one}, f(\text{pred}(n)) * n)$$

**Uninterpreted Solution**

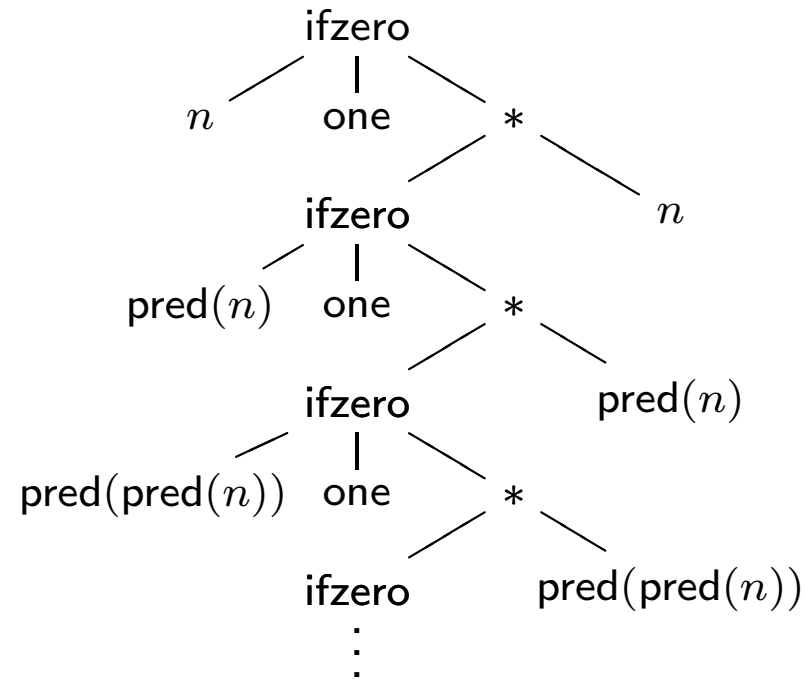

# Example: Signature + Equations

**RPS**

$$\varphi(x, y) \approx F(x, y, \varphi(Gx, Gy))$$

and  $F(x, y, z) = F(y, x, z)$  in any interpretation  $(\implies \varphi \text{ commutative})$

**Uninterpreted solution**

$$\varphi^\dagger(x, y) =$$

```
graph TD; F1[F] --- L1["{ x, y }"]; F1 --- F2[F]; F2 --- L2["{ Gx, Gy }"]; F2 --- F3[F]; F3 --- L3["{ GGx, GGy }"]; F3 -.- Dots["..."]
```

# Interpreted Semantics of RPS

## Classically:

$\Sigma$  given functions

$\Phi$  recursively defined functions

formal equations:  $f(\vec{x}) \approx t^f(\vec{x}), \quad f \in \Phi.$

## and

*suitable*  $\Sigma$ -Algebra  $A \rightsquigarrow$  Interpreted semantics:  $f_A : A^n \rightarrow A, \quad f \in \Phi,$  such that  
formal equations are valid identities

# Interpreted Semantics of RPS

## Classically:

$\Sigma$  given functions  
 $\Phi$  recursively defined functions

formal equations:  $f(\vec{x}) \approx t^f(\vec{x}), \quad f \in \Phi.$

and

*suitable*  $\Sigma$ -Algebra  $A \rightsquigarrow$  Interpreted semantics:  $f_A : A^n \rightarrow A, \quad f \in \Phi,$  such that formal equations are valid identities

## Suitable Algebras

iteration algebras (Bloom & Ésik 1993)

(completely) iterative algebras  
(Nelson 1983, Milius 2005)

reduction to simple  
equations

completely metrizable algebras  
(Arnold & Nivat 1980)

finite approximations

continuous algebras  
(Guessarian 1981)

Common feature: a **canonical evaluation**  $T_\Sigma A \longrightarrow A$  of all  $\Sigma$ -trees.

# Complete Elgot Algebras

**Theorem.** Let  $H : \mathcal{A} \longrightarrow \mathcal{A}$  be an endofunctor (with enough final coalgebras):  
Complete Elgot algebras  $\cong$  Eilenberg-Moore algebra for  $T^H$ .



# Complete Elgot Algebras

**Theorem.** Let  $H : \mathcal{A} \longrightarrow \mathcal{A}$  be an endofunctor (with enough final coalgebras):  
Complete Elgot algebras  $\cong$  Eilenberg-Moore algebra for  $T^H$ .

**Definition.**  $(A, a, (-)^*)$  is a **complete Elgot algebra** for  $H$  if

- (i)  $a : HA \longrightarrow A$  is a  $H$ -algebra,
- (ii)  $(-)^*$  assigns **solutions** to **flat equations** subject to 2 simple axioms

# Complete Elgot Algebras

**Theorem.** Let  $H : \mathcal{A} \longrightarrow \mathcal{A}$  be an endofunctor (with enough final coalgebras):  
Complete Elgot algebras  $\cong$  Eilenberg-Moore algebra for  $T^H$ .

**Definition.**  $(A, a, (-)^*)$  is a **complete Elgot algebra** for  $H$  if

- (i)  $a : HA \longrightarrow A$  is a  $H$ -algebra,
- (ii)  $(-)^*$  assigns **solutions** to **flat equations** subject to 2 simple axioms

**Examples.**

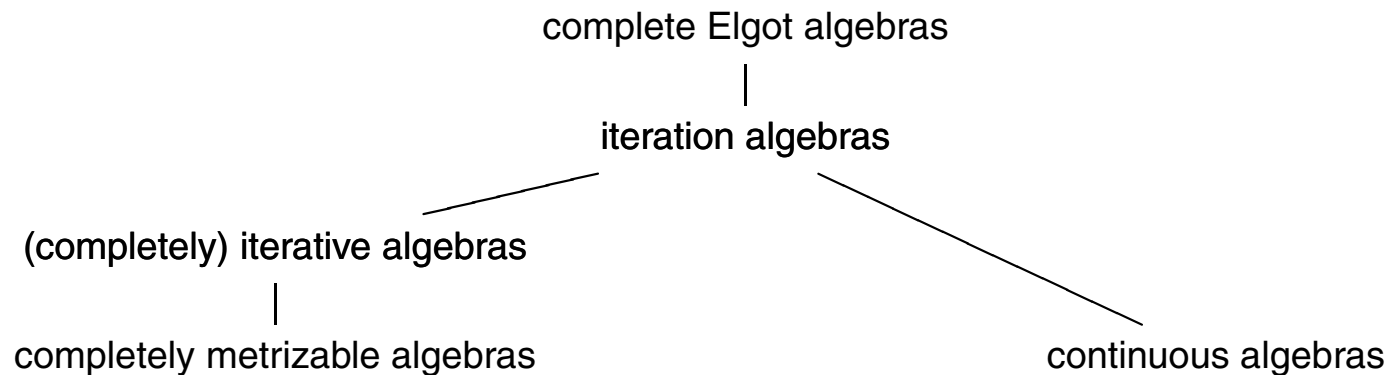

**Note.**  
 $a : HA \longrightarrow A$  completely iterative algebra :  $\iff A$  has **unique** solutions of flat equations.

# Interpreted Solutions of RPS

**Notation.**  $(A, a, (-)^*)$  complete Elgot algebra  $\rightsquigarrow \tilde{a} : T^H A \longrightarrow A$  Eilenberg-Moore alg.

**Assumptions.**  $e : V \longrightarrow T^{H+V}$  guarded RPS;  $(A, a, (-)^*)$  complete Elgot  $H$ -algebra

# Interpreted Solutions of RPS

**Notation.**  $(A, a, (-)^*)$  complete Elgot algebra  $\rightsquigarrow \tilde{a} : T^H A \longrightarrow A$  Eilenberg-Moore alg.

**Assumptions.**  $e : V \longrightarrow T^{H+V}$  guarded RPS;  $(A, a, (-)^*)$  complete Elgot  $H$ -algebra

**Definition.** *Interpreted solution of  $e$  in  $A$ :*  $e_A^\dagger : VA \longrightarrow A$  such that

- (i)  $e_A^\dagger$  can be used in subsequent RPSs as givens;
- (ii) “formal equations are turned into identities in  $A$ ”.

# Interpreted Solutions of RPS

**Notation.**  $(A, a, (-)^*)$  complete Elgot algebra  $\rightsquigarrow \tilde{a} : T^H A \longrightarrow A$  Eilenberg-Moore alg.

**Assumptions.**  $e : V \longrightarrow T^{H+V}$  guarded RPS;  $(A, a, (-)^*)$  complete Elgot  $H$ -algebra

**Definition.** *Interpreted solution of  $e$  in  $A$ :*  $e_A^\dagger : VA \longrightarrow A$  such that

(i)  $[a, e_A^\dagger] : (H + V)A \longrightarrow A$  complete Elgot algebra for  $H + V$

(ii)

$$\begin{array}{ccc}
 VA & \xrightarrow{e_A^\dagger} & A \\
 e_A \downarrow & \nearrow [a, e_A^\dagger] & \\
 T^{H+V}A & & 
 \end{array}$$

# Interpreted Solutions of RPS

**Notation.**  $(A, a, (-)^*)$  complete Elgot algebra  $\rightsquigarrow \tilde{a} : T^H A \longrightarrow A$  Eilenberg-Moore alg.

**Assumptions.**  $e : V \longrightarrow T^{H+V}$  guarded RPS;  $(A, a, (-)^*)$  complete Elgot  $H$ -algebra

**Definition.** *Interpreted solution* of  $e$  in  $A$ :  $e_A^\dagger : VA \longrightarrow A$  such that

(i)  $[a, e_A^\dagger] : (H + V)A \longrightarrow A$  complete Elgot algebra for  $H + V$

(ii)

$$\begin{array}{ccc}
 VA & \xrightarrow{e_A^\dagger} & A \\
 e_A \downarrow & \nearrow [a, e_A^\dagger] & \\
 T^{H+V}A & & 
 \end{array}$$

**Theorem.**

There exists a canonical interpreted solution  $e_A^\dagger$  (called **standard interpreted solution**).

$A$  completely iterative algebra  $\implies e_A^\dagger$  is the **unique** interpreted solution.

# Application: Classical Interpreted Solutions

**RPS**  $f(n) \approx \text{ifzero}(n, \text{one}, f(\text{pred}(n)) * n)$

**Algebra**  $\mathbb{N}_\perp$  with continuous operations

there is a continuous operator  $\text{CPO}(\mathbb{N}_\perp, \mathbb{N}_\perp)$   $\bigcirc_R$  such that  $\mu R = \text{fac} : \mathbb{N}_\perp \longrightarrow \mathbb{N}_\perp$ .

# Application: Classical Interpreted Solutions

**RPS**  $f(n) \approx \text{ifzero}(n, \text{one}, f(\text{pred}(n)) * n)$

**Algebra**  $\mathbb{N}_\perp$  with continuous operations

there is a continuous operator  $\text{CPO}(\mathbb{N}_\perp, \mathbb{N}_\perp) \overset{\curvearrowright}{\circlearrowleft} R$  such that  $\mu R = \text{fac} : \mathbb{N}_\perp \longrightarrow \mathbb{N}_\perp$ .

**Theorem.** For any guarded RPS and any continuous algebra  $A$  there is a continuous operator  $R$  such that

Least fixed point of  $R \quad \equiv \quad \text{standard interpreted solution } e_A^\ddagger$ .

**Note.** This works for suitable *functors* on the category of CPOs.



# Application: Complete Metric Spaces

**RPS**

$$\varphi(x) \approx F(x, \varphi(Gx))$$

**Algebra**

$$A = [0, 1] \quad F_A(a, b) = \frac{a+b}{4} \quad G_A(a) = \frac{\sin a}{2}$$

**Uninterpreted Solution**

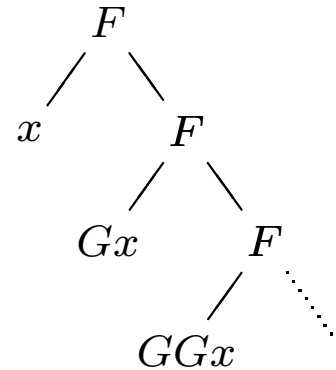

**Interpreted Solution**

unique contraction  $\varphi_A : [0, 1] \longrightarrow [0, 1]$  such that

$$\varphi_A(x) = \frac{1}{4} \left( x + \varphi_A \left( \frac{\sin x}{2} \right) \right)$$

# Application: Complete Metric Spaces

**RPS**

$$\varphi(x) \approx F(x, \varphi(Gx))$$

**Algebra**

$$A = [0, 1] \quad F_A(a, b) = \frac{a+b}{4} \quad G_A(a) = \frac{\sin a}{2}$$

**Uninterpreted Solution**

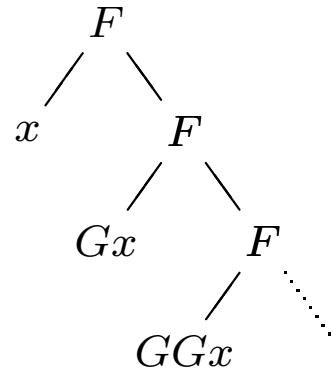

**Interpreted Solution**

unique contraction  $\varphi_A : [0, 1] \longrightarrow [0, 1]$  such that

$$\varphi_A(x) = \frac{1}{4} \left( x + \varphi_A \left( \frac{\sin x}{2} \right) \right)$$

**Theorem.** For any guarded RPS interpreted in a completely metrizable algebra  $A$  there exists a unique interpreted solution  $e_A^\dagger$ .

# Application: Fractals

**RPS**

$$\varphi(x) \approx F(\varphi(x), x, \varphi(x))$$

**Algebra**

$$A = C([0, 1] \times [0, 1]) \quad F_A : \begin{array}{ccc} A \times A \times A & \longrightarrow & A \\ (U, V, W) & \longmapsto & f[U] \cup g[V] \cup h[W] \end{array}$$

$$f(a, b) = \left(\frac{1}{3}a, \frac{1}{3}b\right) \quad g(a, b) = \left(\frac{1}{3}a + \frac{1}{3}, \frac{1}{3}b\right) \quad h(a, b) = \left(\frac{1}{3}a + \frac{2}{3}, \frac{1}{3}b\right)$$

**Uninterpreted Solution**

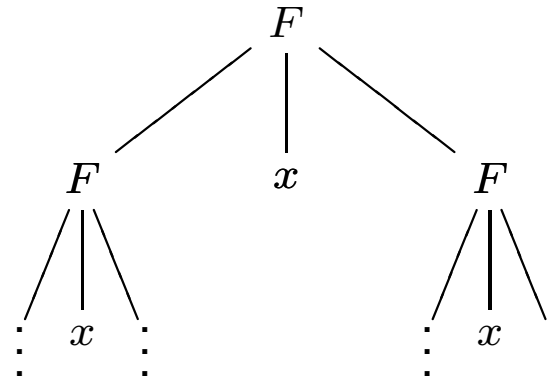

**Interpreted Solution**

unique  $\frac{1}{3}$ -contractive function  $\varphi_A : A \longrightarrow A$ :

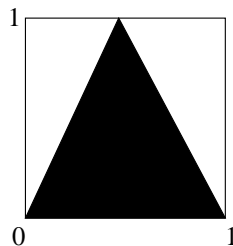

$\xrightarrow{\varphi_A}$

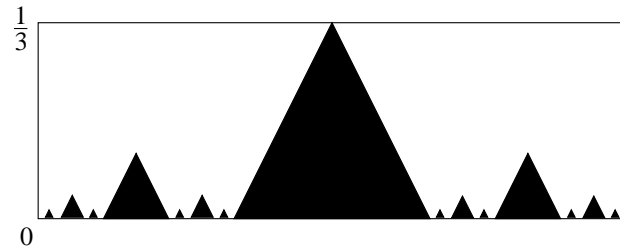

# Application: Non-well founded sets

## RPS

$$\varphi(x) \approx F(x, \varphi(Gx))$$

## Algebra

$HF_1$  = all hereditarily finite sets

$$F_A(u, v) = \{u, u \times v\} \quad G_A(u) = \{\bigcup u\}$$

## Uninterpreted Solution

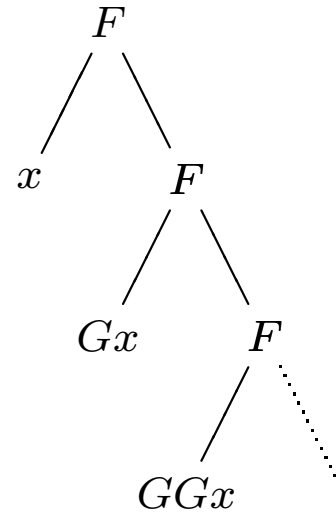

## Interpreted Solution

unique function  $\varphi_A : HF_1 \longrightarrow HF_1$  with

$$\varphi_A(u) = \left\{ u, u \times \varphi_A\left(\{\bigcup u\}\right) \right\}$$

# Consistency

**Example.**  $\varphi(x) \approx F(x, \varphi(Gx))$  **and**  $A \times A \xrightarrow{F_A} A \xleftarrow{G_A} A$  with  $\alpha : T_\Sigma A \longrightarrow A$

canonical evaluation

$$\text{For all } a \in A: \quad \underset{\substack{\uparrow \\ \text{interpreted solution}}}{\varphi_A(a)} = \underset{\substack{\downarrow \\ \text{uninterpreted solution}}}{\alpha} \left( \underbrace{\varphi^\dagger(x)}_{\uparrow} [x := a] \right).$$

# Consistency

**Example.**  $\varphi(x) \approx F(x, \varphi(Gx))$  **and**  $A \times A \xrightarrow{F_A} A \xleftarrow{G_A} A$  with  $\alpha : T_\Sigma A \longrightarrow A$

canonical evaluation

$$\begin{array}{ccc} \text{For all } a \in A: & \varphi_A(a) & = & \alpha \left( \underbrace{\varphi^\dagger(x)}_{\substack{\uparrow \\ \text{uninterpreted solution}}} [x := a] \right) \\ & \uparrow & & \\ & \text{interpreted solution} & & \end{array}$$

**Theorem.**

$e : V \longrightarrow T^{H+V}$  guarded RPS;  $(A, a, (-)^*)$  complete Elgot algebra for  $H$

$e^\dagger : V \longrightarrow T^H$  unique uninterpreted solution

$e_A^\ddagger : VA \longrightarrow A$  standard interpreted solution

Then

$$\begin{array}{ccc} VA & \xrightarrow{(e^\dagger)_A} & T^H A \\ & \searrow e_A^\ddagger & \downarrow \tilde{a} \\ & & A \end{array}$$

# Conclusions

- Coalgebras model various types of systems and provide semantic domains for system behaviour;
- Parameterized final coalgebras have a monad structure, and this gives the free completely iterative monad;
- (Generalized) recursive function definitions and their solutions have a neat categorical formulation;
- Uninterpreted solutions using final coalgebras;
- Interpreted solutions using complete Elgot algebras;
- Applications: various implicit function definitions (CPOs, CMSs, non-well founded sets, signatures+equations ... );
- Consistency of both semantics.

# References

## Coalgebras

- [1] J. Rutten, Universal coalgebra: a theory of systems, *Theoret. Comput. Sci.* 249 (2000), 3–80.
- [2] P. Aczel, A final coalgebra theorem, *Lecture Notes in Comput. Sci.* 389 (1989), 357–365.
- [3] M. Barr, Terminal coalgebras in well-founded set theory, *Theoret. Comput. Sci.* 114 (1993), 299–315.
- [4] J. Worrell, On the final sequence of a finitary set functor, *Theoret. Comput. Sci.* 338 (2005), 184–199.
- [5] J. Adámek, S. Milius, J. Velebil: A General Final Coalgebra Theorem, *Math. Structures Comput. Sci.* 15 (2005), 409–432.
- [6] J. Adámek, S. Milius, J. Velebil: On coalgebra bases on classes, *Theoret. Comput. Sci.* 316 (2004), 3–23.

## Monads & Semantics

- [1] L. S. Moss, Parametric Corecursion, *Theoret. Comput. Sci.* 260 (2001), 139–163.
- [2] N. Ghani, C. Lüth, F. De Marchi, J. Power, Dualizing initial algebras, *Math. Structures Comput. Sci.* 13 (2003), 349–370.
- [3] P. Aczel, J. Adámek, S. Milius, J. Velebil: Infinite trees and completely iterative theories: a coalgebraic view, *Theoret. Comput. Sci.* 300 (2003), 1–45.
- [4] S. Milius, Completely Iterative Algebras and Completely Iterative Monads, *Inform. and Comput.* 196 (2005), 1–41.
- [5] N. Ghani, C. Lüth, F. De Marchi, Solving algebraic equations using coalgebra, *Theor. Inform. Appl.* 37 (2003), 301–314.
- [6] J. Adámek, S. Milius, J. Velebil: Elgot Algebras, accepted for publication in *Logical Methods Comput. Sci.*
- [7] S. Milius, L. S. Moss: The Category Theoretic Solution of Recursive Program Schemes, to appear in *Theoret. Comput. Sci.*
